# Supplementary material for: Unsupervised Contrastive Learning for Robust RF Device Fingerprinting Under Time-Domain Shift
Source: arXiv:2403.04036 source file (2024-03-06)
Supplement: Supplementary file 1 [file appendix.tex]

%%% ---------------- x ---------------- %%%
%% -------- x -------- %%
% ---- x ---- %

%%% ---------------- Appendix ---------------- %%%

% \subsection{Appendix Table} \label{sec:tb}
% Move this part to Appendix Section.
% The table includes the real testing accuracy of the 4 \emph{Set}s (S1, S4, S5, S6). The exact results need to be regenerated. 

\subsection{Detailed Results on Wired RF Data} \label{sec:wdres}

% -------- Table: Wired D1 <-> D2 -------- %  
% \begin{table}[!htb]
%     \centering \resizebox{0.95\columnwidth}{!}{
%       \begin{tabular}{@{}l|lll|lll@{}}
%         \toprule
%         \multicolumn{1}{l|}{\thead{Wired (Source $\rightarrow$ Target)}} & \multicolumn{3}{l|}{\thead{Day 1 $\rightarrow$ 2}} & \multicolumn{3}{l}{\thead{Day 2 $\rightarrow$ 1}} \\
%         \toprule
%         \#Device K = 16 & CNN & AB & CTL & CNN & AB & CTL \\
%         \midrule
%         DayA\_S1  $\rightarrow$ DayB\_S1 & 50.4 & 57.8 & 71.9 & 67.5 & 46.0 & 78.8\\
%         DayA\_S1  $\rightarrow$ DayB\_S2 & 51.6 & 58.2 & 71.0 & 65.1 & 45.4 & 75.4\\
%         DayA\_S1  $\rightarrow$ DayB\_S3 & 53.6 & 57.9 & 67.6 & 66.5 & 42.8 & 76.4\\
%         DayA\_S1  $\rightarrow$ DayB\_S4 & 52.4 & 60.9 & 77.2 & 66.9 & 42.8 & 78.6\\
%         \bottomrule
%       \end{tabular}
%     }
%     \caption{Detailed classification accuracy of domain adaptation between one \emph{Set} of day 1 and another \emph{Set} of day 2 on \textbf{wired} RF devices under baseline model (CNN), ablation model (AB), and contrastive model (CTL).}
%     \label{tab:expr_tb_wired}
%   \end{table}

% -------- Confusion Matrix: Wired D1 <-> D2 -------- %  
\comment{
\begin{figure}
    \centering 
    \subfloat[CNN, Day 1 $\rightarrow$ 2]{%
      \includegraphics[width=0.16\textwidth]{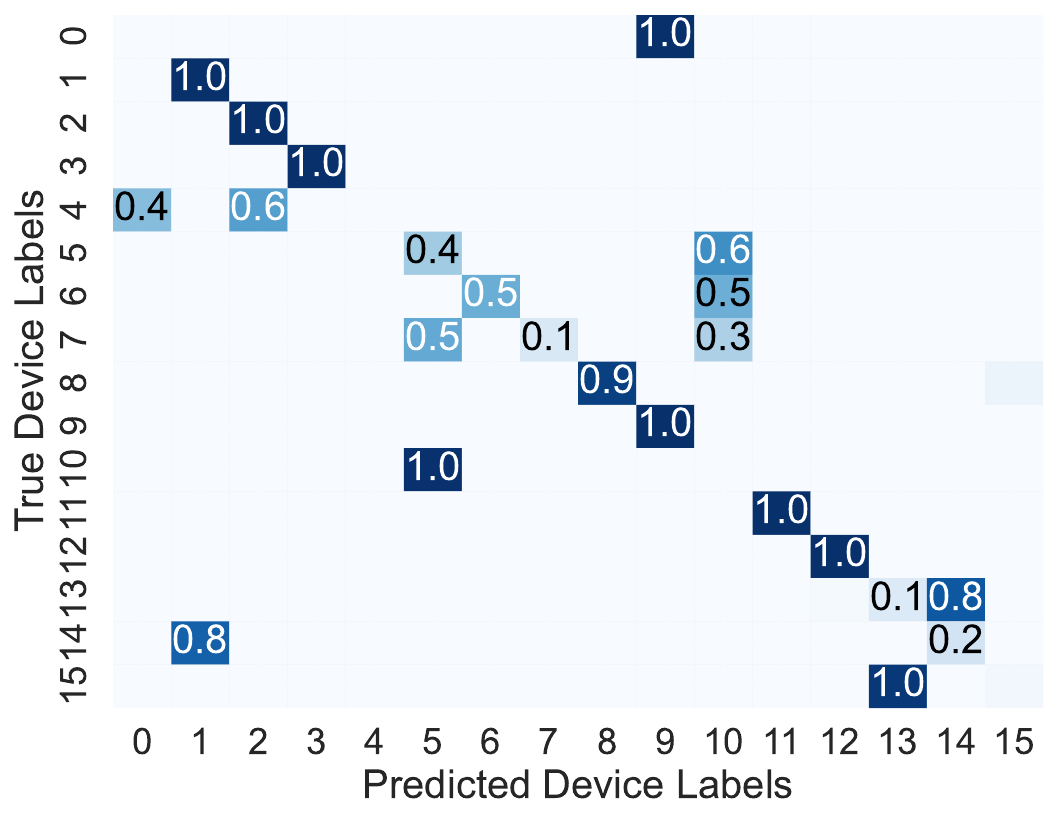}
      \label{fig:expr_cm_cnn_wired12}} \hspace*{-0.5em} 
    \subfloat[AB, Day 1 $\rightarrow$ 2]{%
      \includegraphics[width=0.16\textwidth]{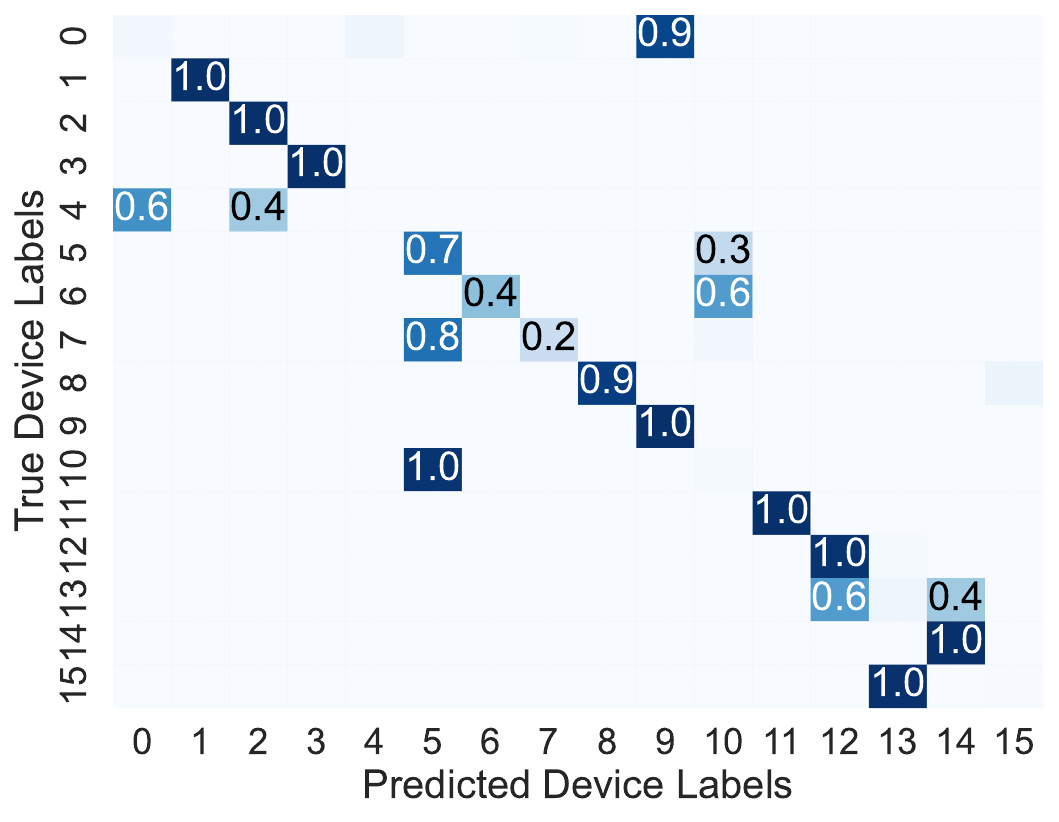}
      \label{fig:expr_cm_ab_wired12}} \hspace*{-0.5em} 
    \subfloat[CTL, Day 1 $\rightarrow$ 2]{%
      \includegraphics[width=0.16\textwidth]{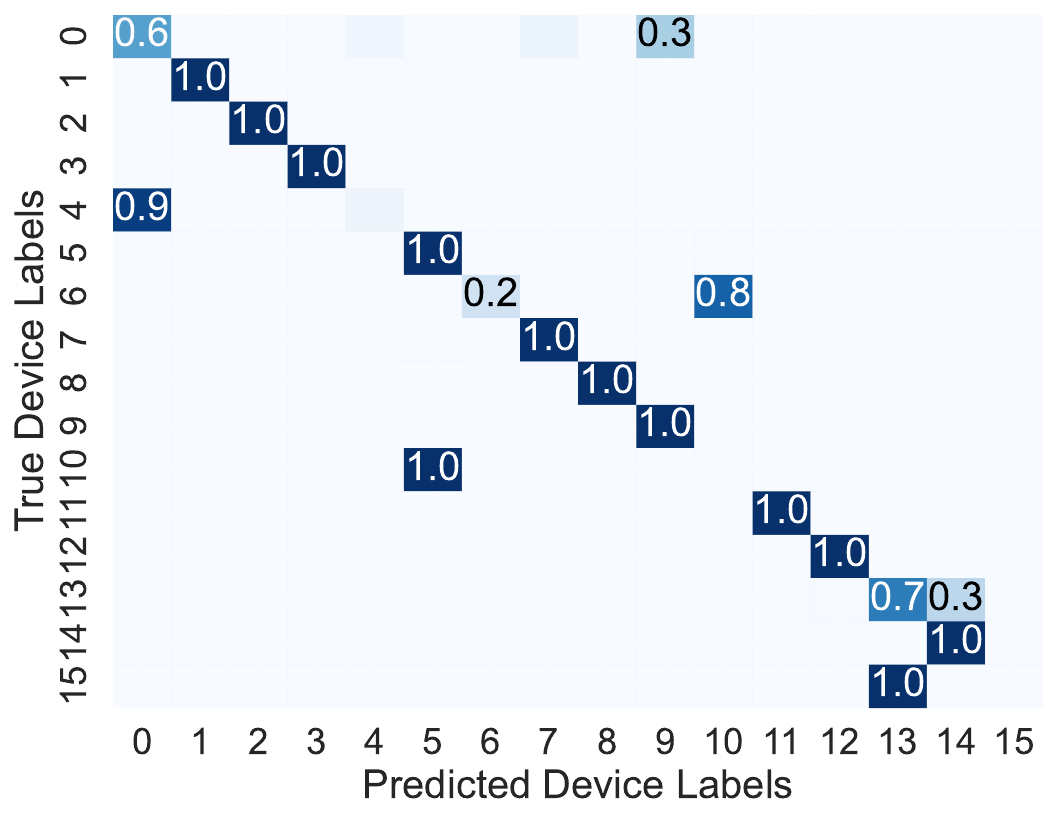}
      \label{fig:expr_cm_ctl_wired12}} \hspace*{-0.5em} 
  \newline
    \subfloat[CNN, Day 2 $\rightarrow$ 1]{%
      \includegraphics[width=0.16\textwidth]{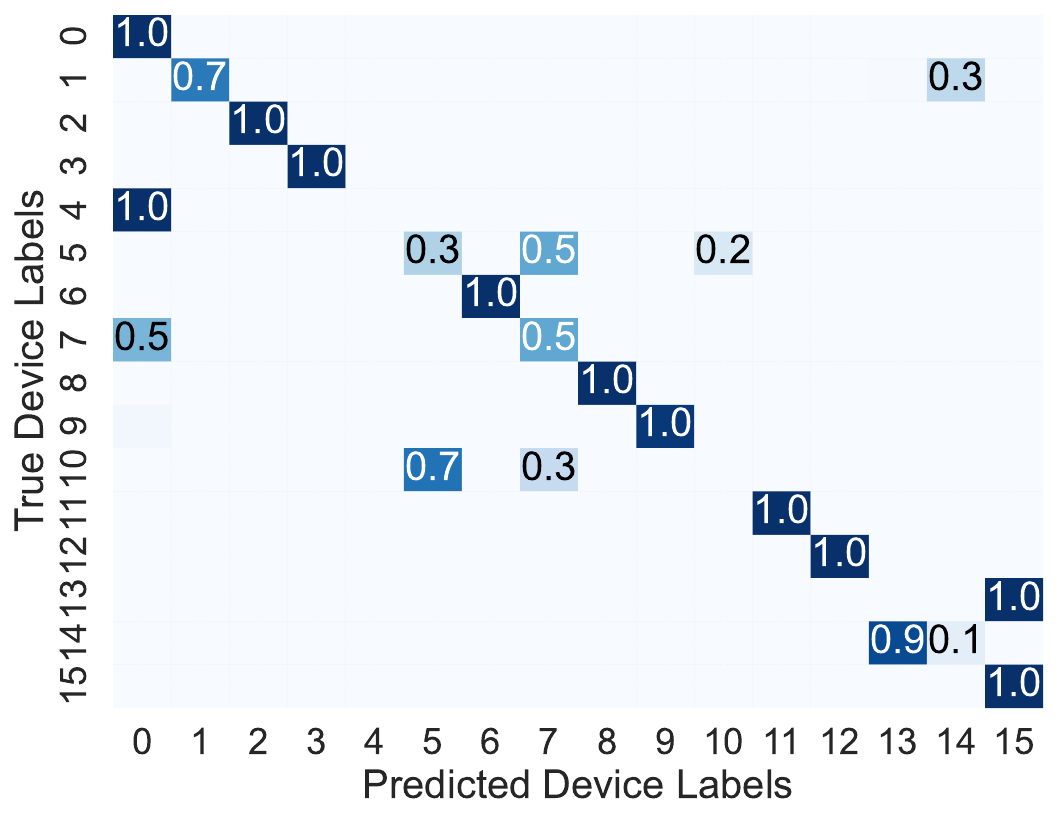}
      \label{fig:expr_cm_cnn_wired21}} \hspace*{-0.5em}
    \subfloat[AB, Day 2 $\rightarrow$ 1]{%
      \includegraphics[width=0.16\textwidth]{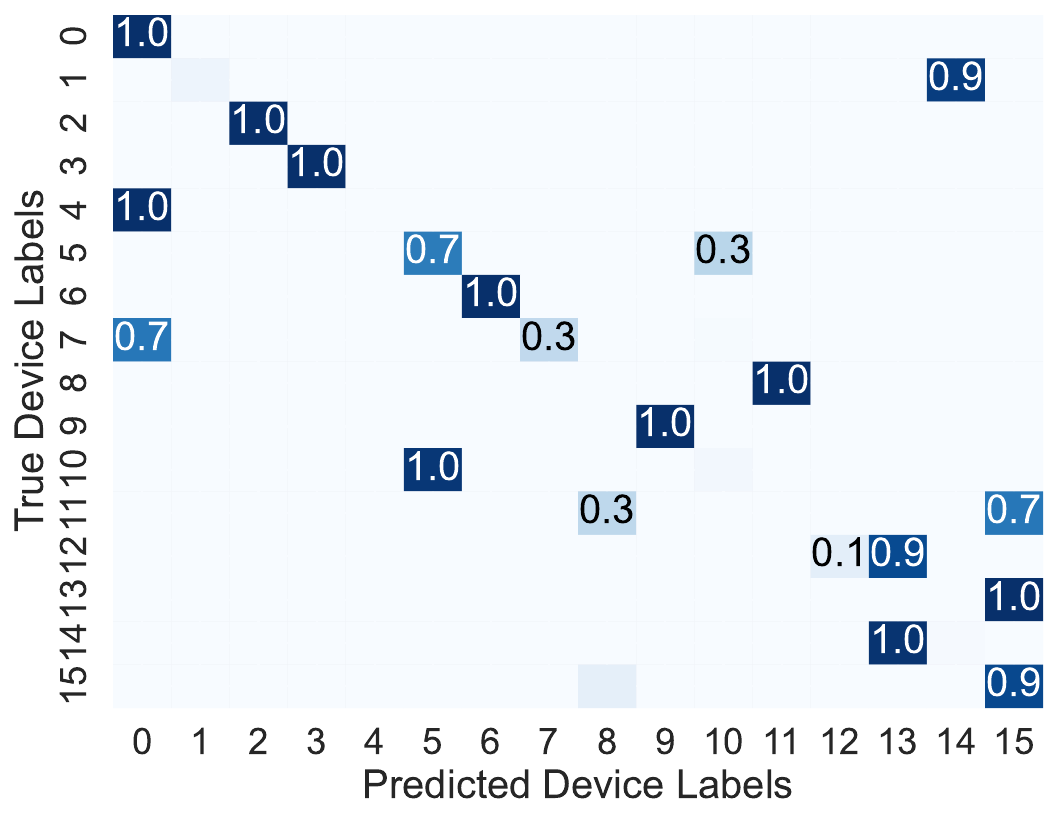}
      \label{fig:expr_cm_ab_wired21}} \hspace*{-0.5em} 
    \subfloat[CTL, Day 2 $\rightarrow$ 1]{%
      \includegraphics[width=0.16\textwidth]{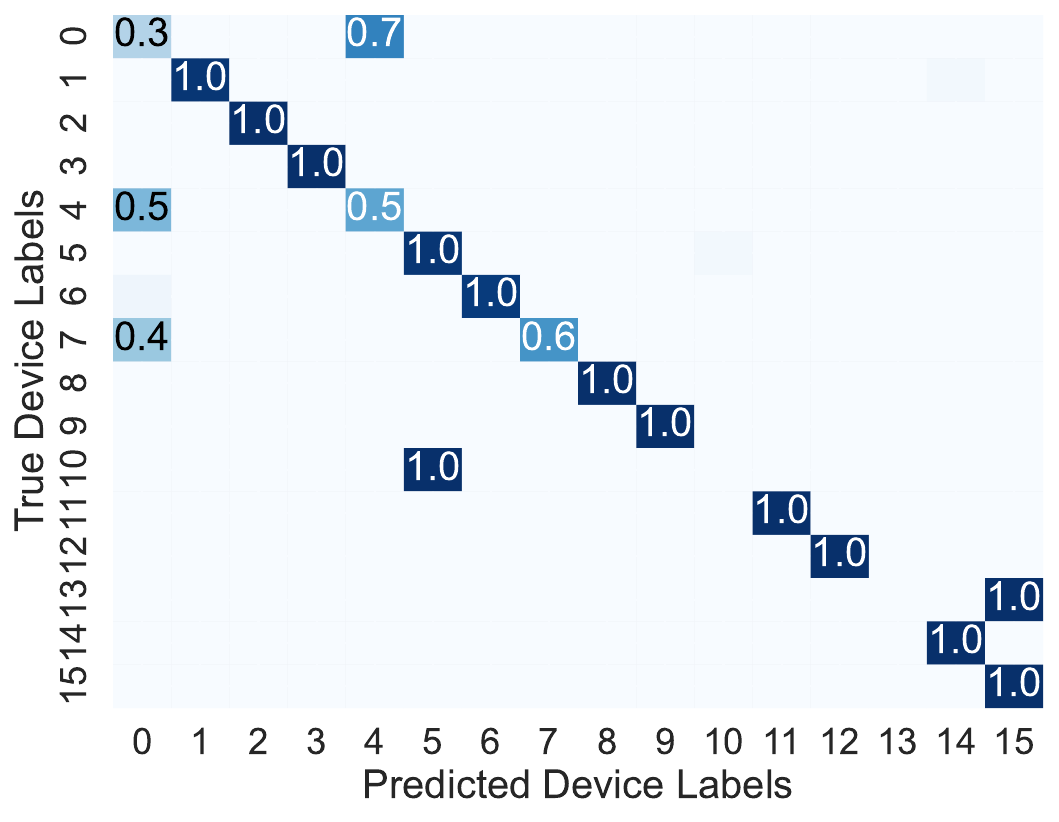}
      \label{fig:expr_cm_ctl_wired21}} \hspace*{-0.5em}
    \caption{Confusion matrix of domain adaptation classification between day 1 and day 2 on \textbf{wired} RF devices for CNN, AB and CTL. The confusion matrix is normalized by row, enabling a clearer visualization of the predicted accuracy distribution across different classes.}
    \label{fig:expr_cm_wired12}
  \end{figure}
}

\subsection{Detailed Results on Wireless RF Data} \label{sec:wlres}

\comment{
\begin{figure}
    \centering 
    \subfloat[CNN, Day 1 $\rightarrow$ 2]{%
      \includegraphics[width=0.16\textwidth]{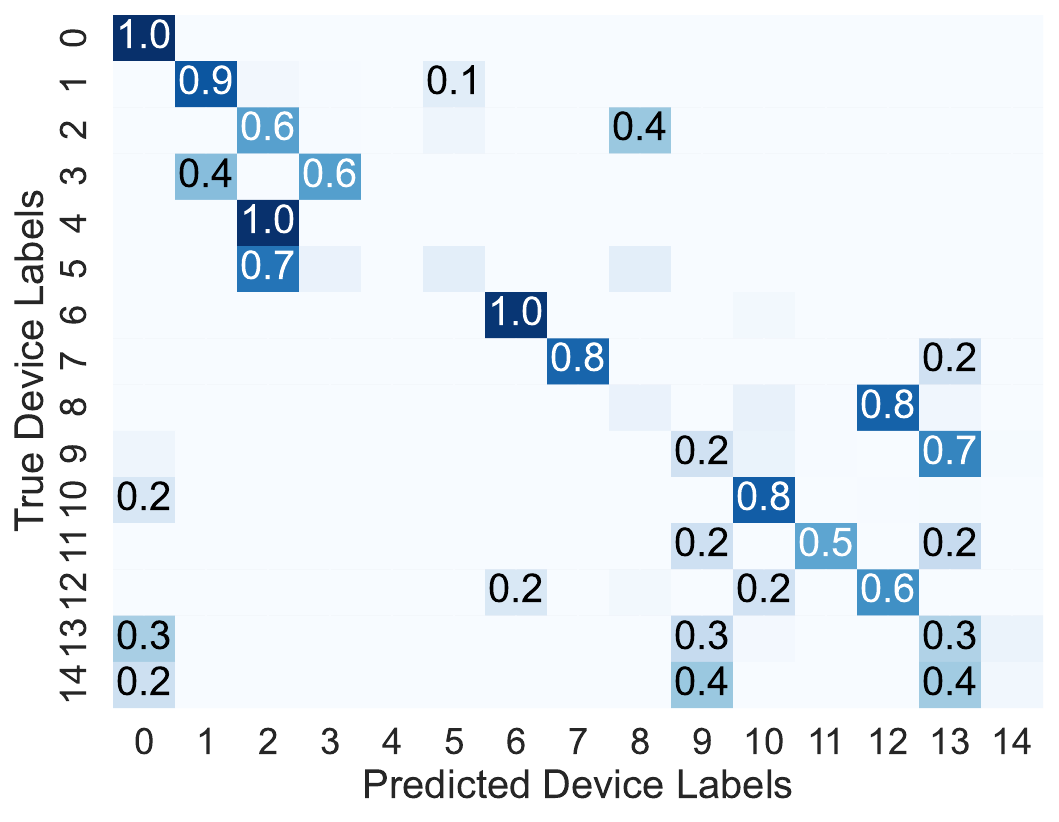}
      \label{fig:expr_cm_cnn_wireless12}} \hspace*{-0.5em} 
    \subfloat[AB, Day 1 $\rightarrow$ 2]{%
      \includegraphics[width=0.16\textwidth]{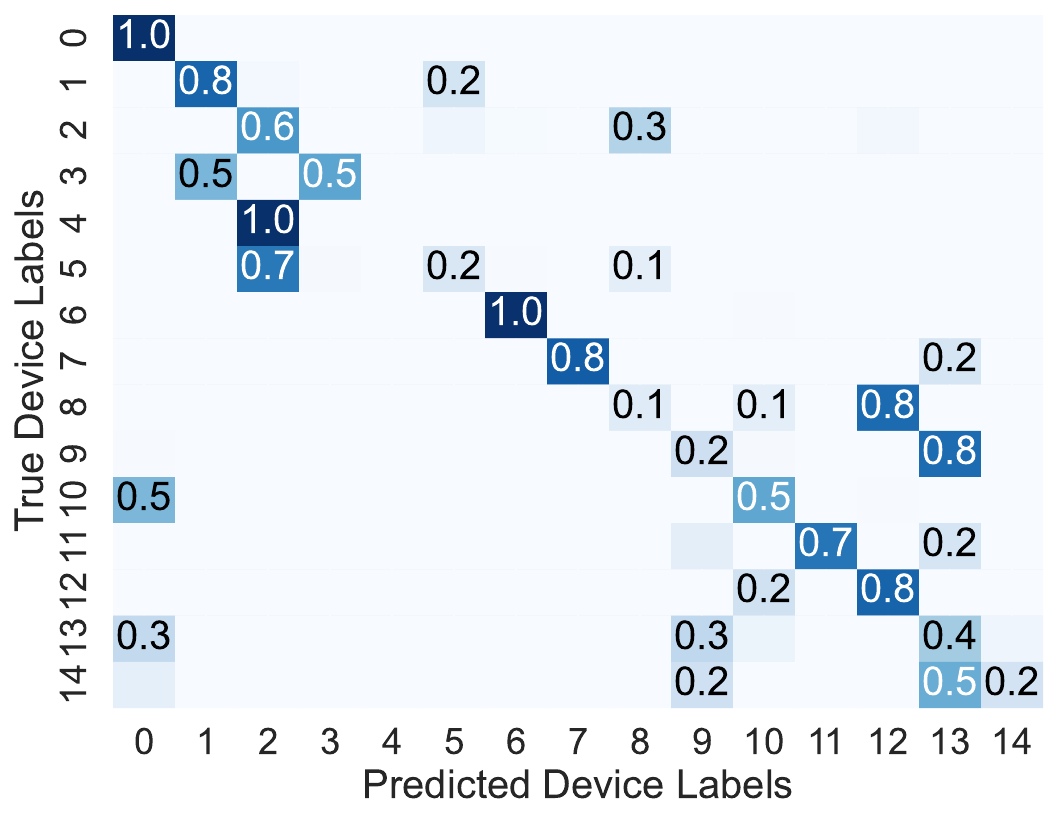}
      \label{fig:expr_cm_ab_wireless12}} \hspace*{-0.5em} 
    \subfloat[CTL, Day 1 $\rightarrow$ 2]{%
      \includegraphics[width=0.16\textwidth]{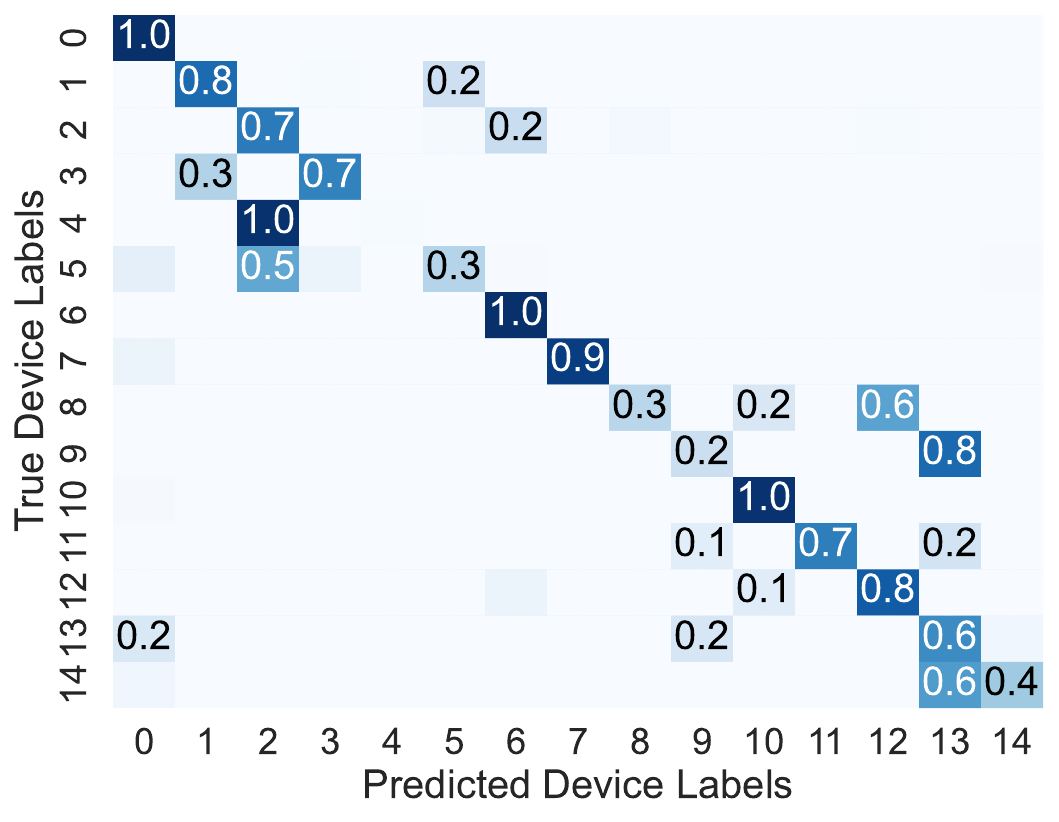}
      \label{fig:expr_cm_ctl_wireless12}} \hspace*{-0.5em} 
  \newline
    \subfloat[CNN, Day 2 $\rightarrow$ 1]{%
      \includegraphics[width=0.16\textwidth]{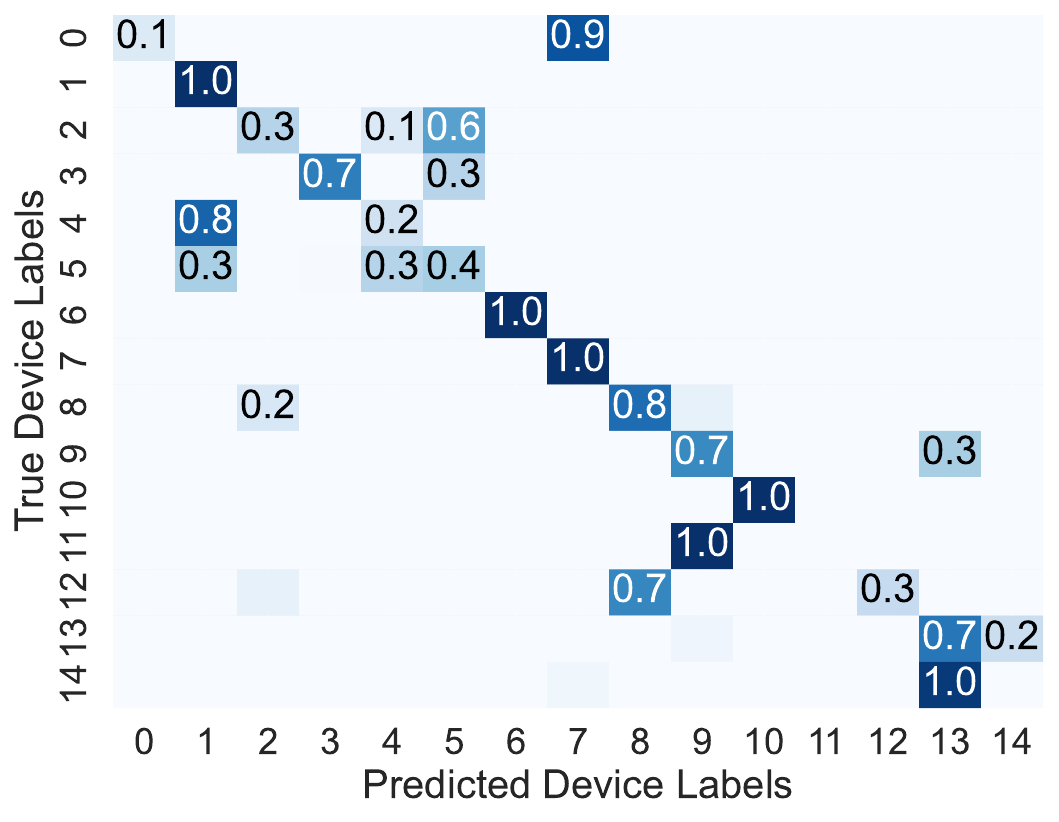}
      \label{fig:expr_cm_cnn_wireless21}} \hspace*{-0.5em}
    \subfloat[AB, Day 2 $\rightarrow$ 1]{%
      \includegraphics[width=0.16\textwidth]{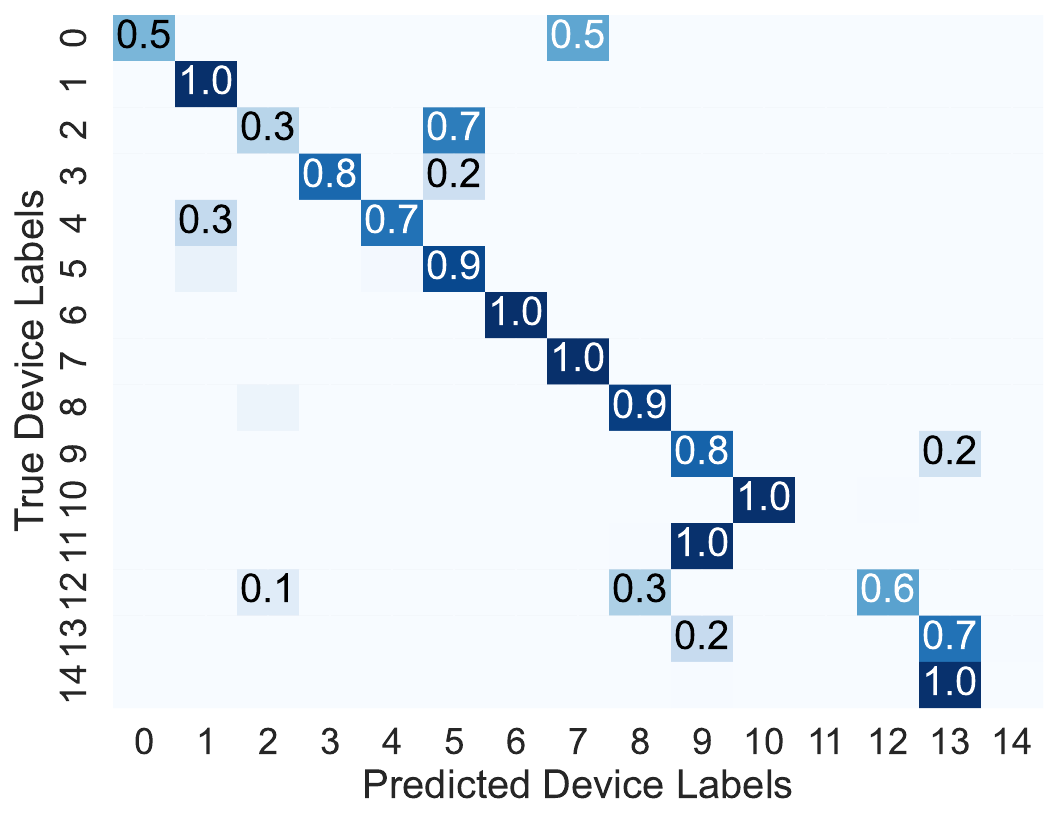}
      \label{fig:expr_cm_ab_wireless21}} \hspace*{-0.5em} 
    \subfloat[CTL, Day 2 $\rightarrow$ 1]{%
      \includegraphics[width=0.16\textwidth]{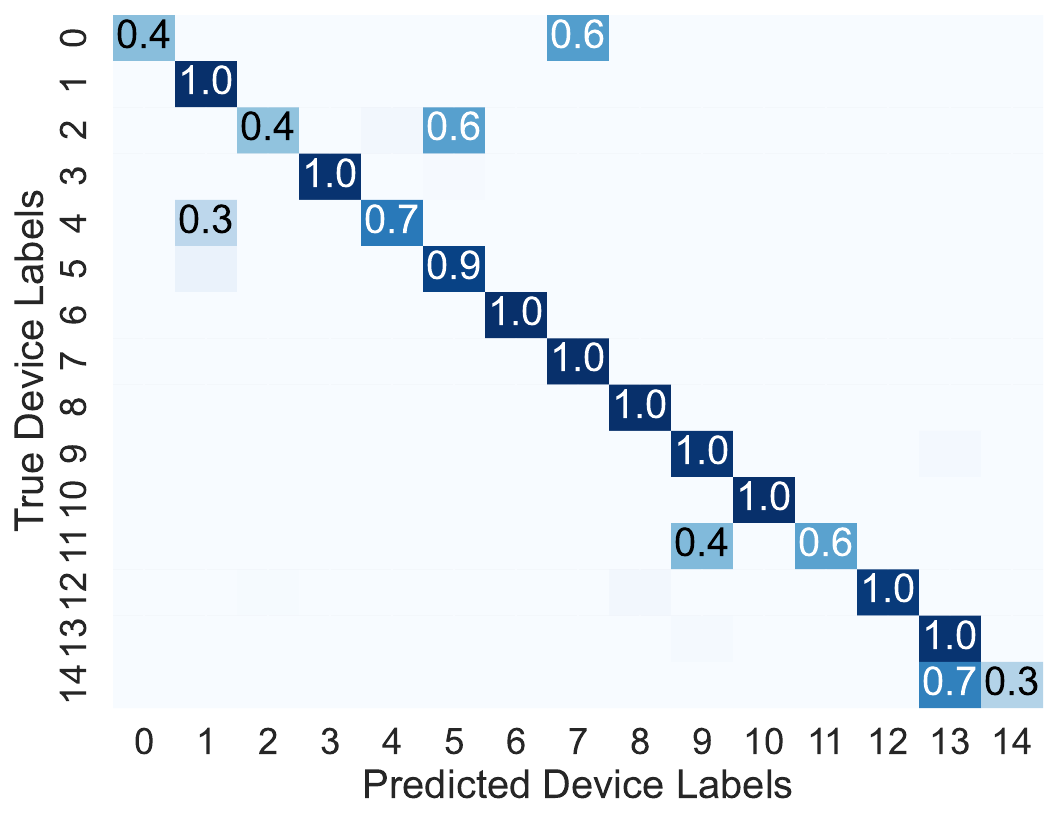}
      \label{fig:expr_cm_ctl_wireless21}} \hspace*{-0.5em}
    \caption{Confusion matrix of domain adaptation classification between day 1 and day 2 on \textbf{wireless} RF devices for CNN, AB and CTL. The confusion matrix is normalized by row, enabling a clearer visualization of the predicted accuracy distribution across different classes.}
    \label{fig:expr_cm_wireless12}
  \end{figure}
}

  % -------- Confusion Matrix: Wireless D2 <-> D3 -------- %  
\comment{
\begin{figure}
    \centering 
    \subfloat[CNN, Day 2 $\rightarrow$ 3]{%
      \includegraphics[width=0.16\textwidth]{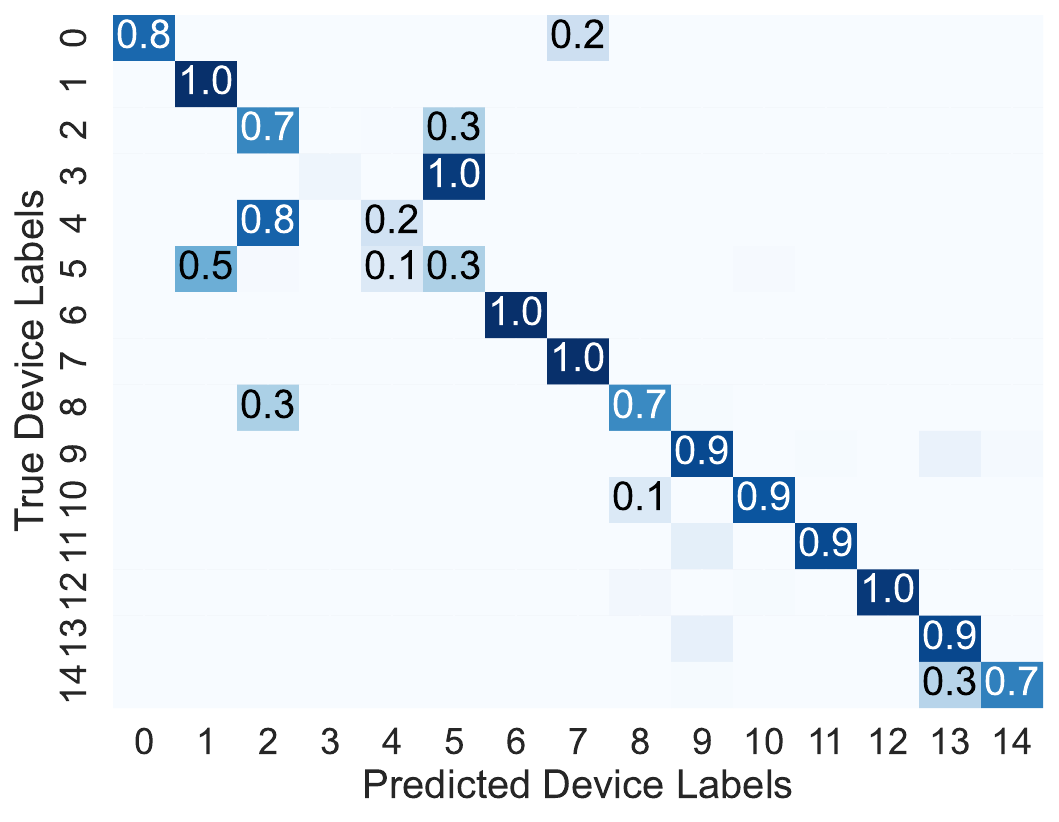}
      \label{fig:expr_cm_cnn_wireless23}} \hspace*{-0.5em} 
    \subfloat[AB, Day 2 $\rightarrow$ 3]{%
      \includegraphics[width=0.16\textwidth]{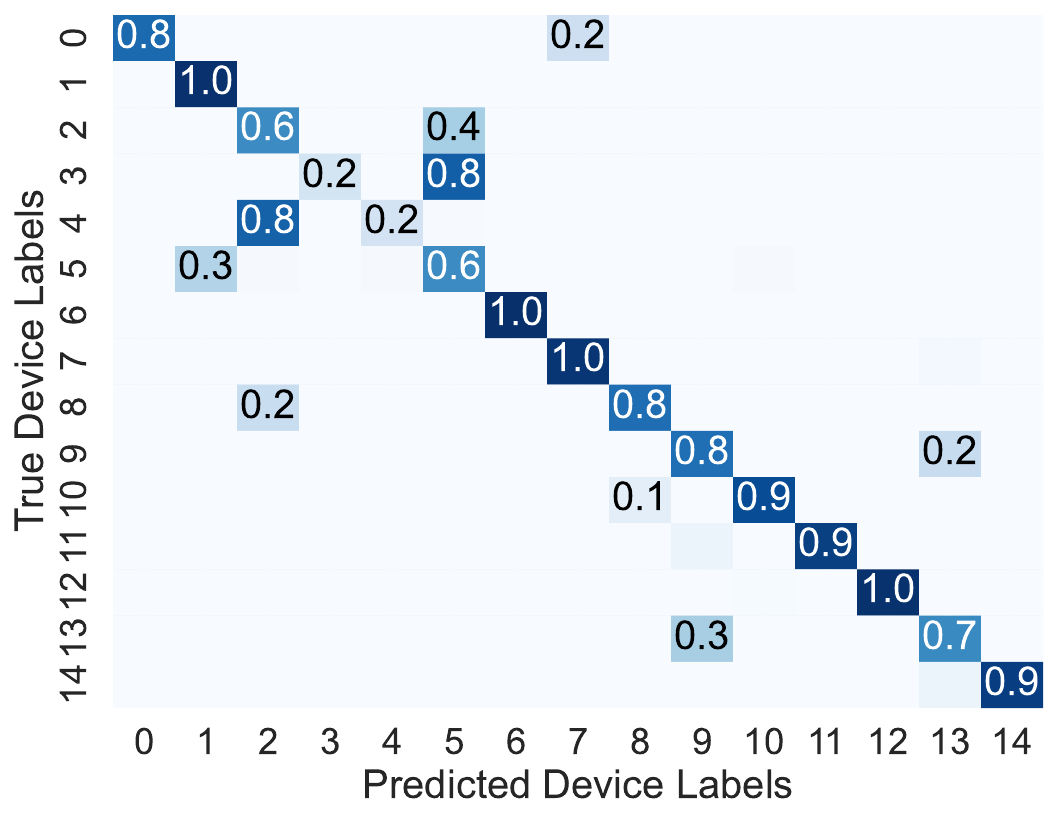}
      \label{fig:expr_cm_ab_wireless23}} \hspace*{-0.5em} 
    \subfloat[CTL, Day 2 $\rightarrow$ 3]{%
      \includegraphics[width=0.16\textwidth]{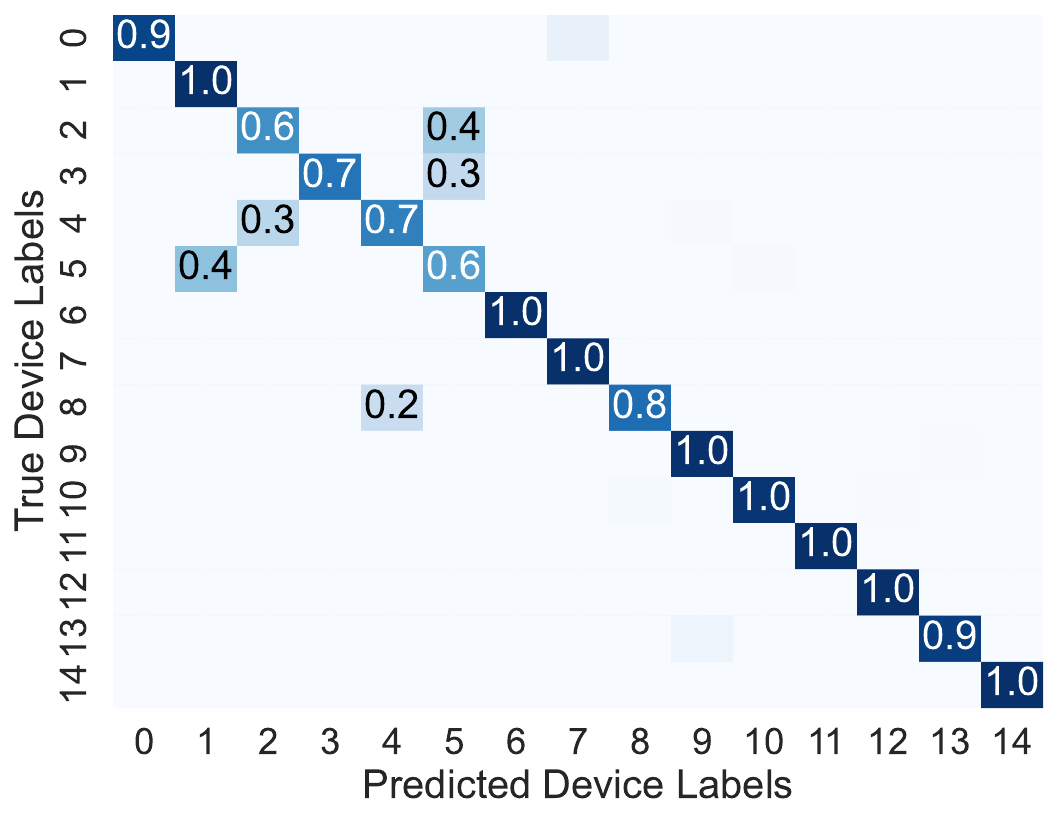}
      \label{fig:expr_cm_ctl_wireless23}} \hspace*{-0.5em} 
  \newline
    \subfloat[CNN, Day 3 $\rightarrow$ 2]{%
      \includegraphics[width=0.16\textwidth]{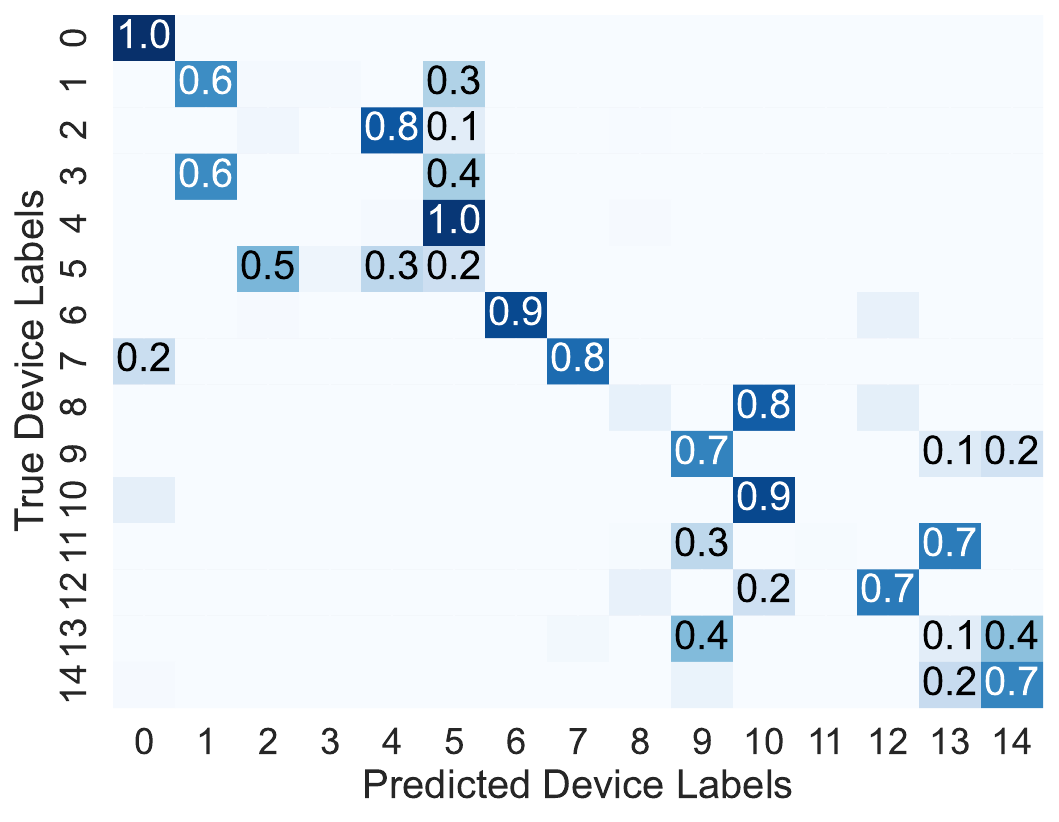}
      \label{fig:expr_cm_cnnwireless32}} \hspace*{-0.5em}
    \subfloat[AB, Day 3 $\rightarrow$ 2]{%
      \includegraphics[width=0.16\textwidth]{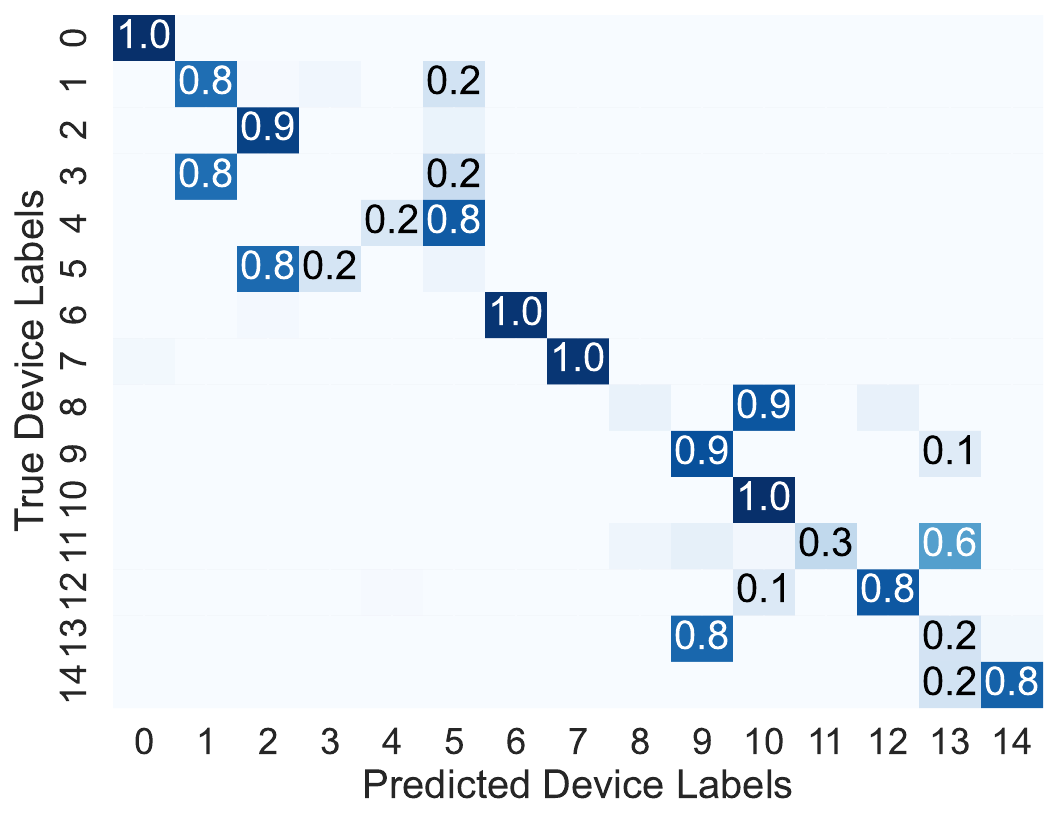}
      \label{fig:expr_cm_ab_wireless32}} \hspace*{-0.5em} 
    \subfloat[CTL, Day 3 $\rightarrow$ 2]{%
      \includegraphics[width=0.16\textwidth]{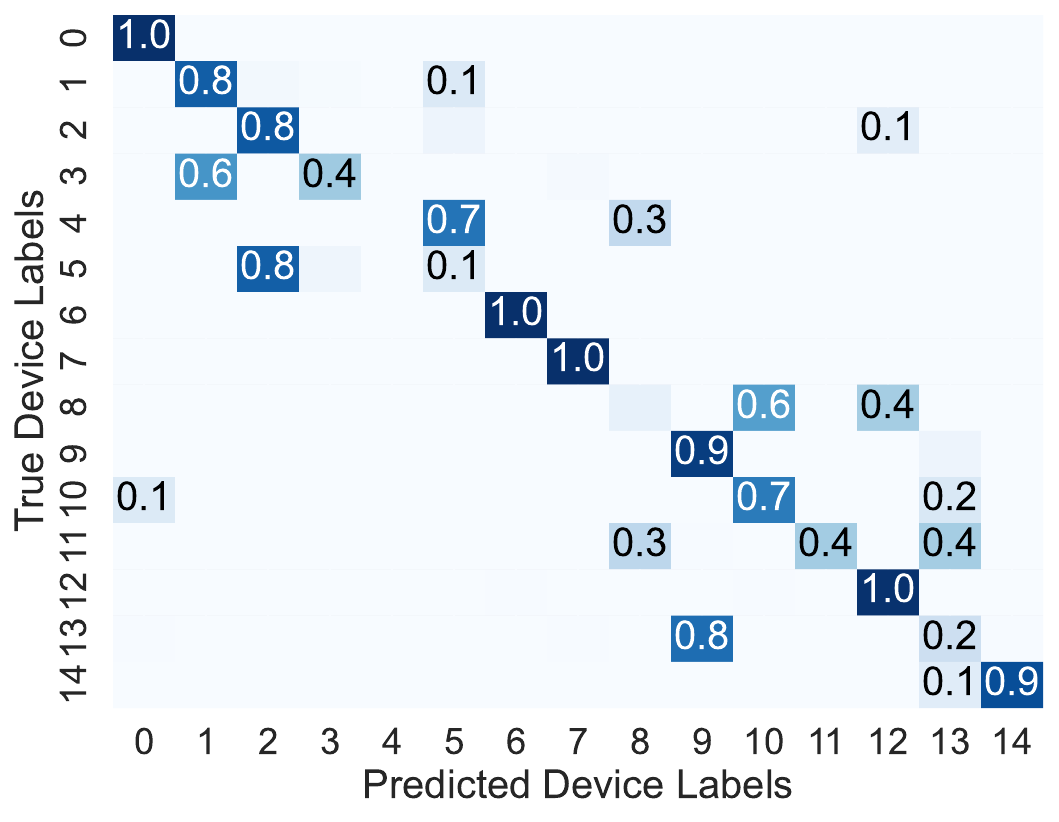}
      \label{fig:expr_cm_ctl_wireless32}} \hspace*{-0.5em}
    \caption{Confusion matrix of domain adaptation classification between day 2 and day 3 on \textbf{wireless} RF devices for CNN, AB and CTL. The confusion matrix is normalized by row, enabling a clearer visualization of the predicted accuracy distribution across different classes.}
    \label{fig:expr_cm_wireless23}
  \end{figure}
}
